# Supplementary material for: Online Decision Mediation
Source: arXiv:2310.18601 source file (2023-10-28)
Supplement: Supplementary file 2 [file supplement.tex]

\newpage
%%%%%%%%%%%%%%%%%%%%%%%%%%%%%%%%%%%%%%%%%%%%%%%%%%%%%%%%%%%%%%%%%%%%%%%%%%%%%%%
\section*{Unweighted Generalization}
%%%%%%%%%%%%%%%%%%%%%%%%%%%%%%%%%%%%%%%%%%%%%%%%%%%%%%%%%%%%%%%%%%%%%%%%%%%%%%%

Loss $\in[a,b]$ (is RV w.r.t. $F$):

\begin{equation}
\ell(f)
\coloneqq
\mathbb{E}_{X\sim\rho_{e}}
\mathcal{L}(\pi_{e}(\cdot|X),\pi_{f}(\cdot|X))
\end{equation}

\begin{equation}
\hat{\ell}(f)
\coloneqq
\mathbb{E}_{X\sim\hat{\rho}_{e}}
\mathcal{L}(\hat{\pi}_{e}(\cdot|X),\pi_{f}(\cdot|X))
\end{equation}

Expected Loss (is RV w.r.t. $D$):

\begin{equation}
l(d)
\coloneqq
\mathbb{E}_{F\sim p(\cdot|d)}
\ell(F)
\end{equation}

\begin{equation}
\hat{l}(d)
\coloneqq
\mathbb{E}_{F\sim p(\cdot|d)}
\hat{\ell}(F)
\end{equation}

Sequence of Datasets:

\begin{equation}
D_{0},...,D_{n},...
\end{equation}

Sequence of Expected Losses:

\begin{equation}
L_{0},...,L_{n},...
\end{equation}

\newpage

Lemma (Donsker-Varadhan):

\begin{equation}
\begin{split}
D_{\subtext{KL}}(p\|q)
&=
\textstyle\sup_{h:\mathcal{F}\rightarrow\mathbb{R}}
\big(
\mathbb{E}_{F\sim p}g(F)
-
\log\mathbb{E}_{F\sim q}e^{g(F)}
\big)
\\
&\geq
\mathbb{E}_{F\sim p}g(F)
-
\log\mathbb{E}_{F\sim q}e^{g(F)}
\end{split}
\end{equation}

\begin{equation}
\begin{split}
\log\mathbb{E}_{F\sim q}e^{g(F)}
&=
\textstyle\sup_{p\in\Delta(\mathcal{F})}\big(
\mathbb{E}_{F\sim p}g(F)
-
D_{\subtext{KL}}(p\|q)
\big)
\\
&\geq
\mathbb{E}_{F\sim p}g(F)
-
D_{\subtext{KL}}(p\|q)
\end{split}
\end{equation}

Lemma (Boucheron-Bennett): Let $\phi(z)\coloneqq e^{z}-z-1$:

\begin{equation}
\begin{split}
e^{\lambda u}-\lambda u-1
&\leq
(e^{(b-a)\lambda}-(b-a)\lambda-1)
\frac{u^{2}}{(b-a)^{2}}
\\
\log\mathbb{E}_{U\sim p}e^{\lambda U}-\mathbb{E}_{U\sim p}\lambda U
\leq
\mathbb{E}_{U\sim p}e^{\lambda U}-\mathbb{E}_{U\sim p}\lambda U-1
&\leq
\phi((b-a)\lambda)\mathbb{E}_{U\sim p}
\frac{U^{2}}{(b-a)^{2}}
\end{split}
\end{equation}

Let $\mathbb{E}_{F\sim p(\cdot|d)}\ell(F)^{2}\leq v$ for all $d$, for some $v$:

\begin{equation}
\begin{split}
(L_{n}-L_{n-1})\lambda
&=
\lambda l(D_{n})-\lambda l(D_{n-1})
\\
&=
\mathbb{E}_{F\sim p(\cdot|D_{n})}
\lambda\ell(F)
-
\mathbb{E}_{F\sim p(\cdot|D_{n-1})}
\lambda\ell(F)
\\
&\leq
\log\mathbb{E}_{F\sim p(\cdot|D_{n-1})}e^{\lambda\ell(F)}
-
\mathbb{E}_{F\sim p(\cdot|D_{n-1})}
\lambda\ell(F)
+
D_{\subtext{KL}}\big(p(\cdot|D_{n})\|p(\cdot|D_{n-1})\big)
\\
&\leq
\phi((b-a)\lambda)
\mathbb{E}_{F\sim p(\cdot|D_{n-1})}\frac{\ell(F)^{2}}{(b-a)^{2}}
+
D_{\subtext{KL}}\big(p(\cdot|D_{n})\|p(\cdot|D_{n-1})\big)
\\
&\leq
\phi((b-a)\lambda)
\frac{v}{(b-a)^{2}}
+
D_{\subtext{KL}}\big(p(\cdot|D_{n})\|p(\cdot|D_{n-1})\big)
\\
L_{n}-L_{n-1}
&\leq
\frac{1}{\lambda}
\Big(
\phi((b-a)\lambda)
\frac{v}{(b-a)^{2}}
+
D_{\subtext{KL}}\big(p(\cdot|D_{n})\|p(\cdot|D_{n-1})\big)
\Big)
\end{split}
\end{equation}

Minimize RHS w.r.t. $\lambda$:

\begin{equation}
\begin{split}
\frac{\partial}{\partial\lambda}
\text{RHS}
&=
0
\\
((b-a)\lambda-1)e^{(b-a)\lambda-1}
&=
\frac{(b-a)^{2}D_{\subtext{KL}}(p(\cdot|D_{n})\|p(\cdot|D_{n-1}))-v}{ve}
\\
\lambda
&=
\frac{1}{b-a}\Big(
W_{0}\Big(
\tfrac{(b-a)^{2}D_{\subtext{KL}}(p(\cdot|D_{n})\|p(\cdot|D_{n-1}))-v}{ve}
\Big)
+1
\Big)
\end{split}
\end{equation}

Define (absolute) ``deterioration upper bound'' (is RV w.r.t. $D_{n},D_{n-1}$):

\begin{equation}
g(D_{n},D_{n-1})
\coloneqq
e^{W_{0}\left(\frac{D_{\subtext{KL}}(p(\cdot|D_{n})\|p(\cdot|D_{n-1}))-1}{e}\right)+1}-1
\end{equation}

and (relative) to some $G_{0}$:

\begin{equation}
\tilde{G}_{n}\coloneqq G_{n}/G_{0}
\end{equation}

Then (plugging in the minimizing $\lambda$) the deterioration is bounded above:

\begin{equation}
\begin{split}
\Delta L_{n}
&\leq
(b-a)G_{n}
\\
\frac{\Delta L_{n}}{(b-a)G_{0}}
&\leq
\tilde{G}_{n}
\end{split}
\end{equation}

Therefore for $\gamma\in(0,1)$:

\begin{equation}
\tilde{G}_{n}\leq\gamma
\implies
\Delta L_{n}\leq\gamma(b-a)G_{0}
\end{equation}

\newpage
%%%%%%%%%%%%%%%%%%%%%%%%%%%%%%%%%%%%%%%%%%%%%%%%%%%%%%%%%%%%%%%%%%%%%%%%%%%%%%%
\section*{Weighted Generalization}
%%%%%%%%%%%%%%%%%%%%%%%%%%%%%%%%%%%%%%%%%%%%%%%%%%%%%%%%%%%%%%%%%%%%%%%%%%%%%%%

Loss $\in[a,b]$ (is RV w.r.t. $Y,\hat{Y}$):

\begin{equation}
\ell(y,\hat{y})
\end{equation}

Expected Loss (is RV w.r.t. $D$):

\begin{equation}
\begin{split}
l(d)
&\coloneqq
\mathbb{E}_{X,Y\sim p_{*}}
\mathbb{E}_{\hat{Y}\sim p(\cdot|d,X)}
\ell(Y,\hat{Y})
\\
\tilde{l}(d)
&\coloneqq
\mathbb{E}_{X,Y\sim\tilde{p}_{*}}
\mathbb{E}_{\hat{Y}\sim p(\cdot|d,X)}
\ell(Y,\hat{Y})
\end{split}
\end{equation}

Sequence of Datasets:

\begin{equation}
D_{0},...,D_{n},...
\end{equation}

Sequence of Expected Losses:

\begin{equation}
L_{0},...,L_{n},...
\end{equation}

%==============================================================================
\textbf{Lemma}.
%==============================================================================

\begin{equation}
\mathbb{E}_{\hat{Y}\sim p(\cdot|d_{n},x)}
\ell(y,\hat{Y})
\leq
\log
\mathbb{E}_{\hat{Y}\sim p(\cdot|d_{n-1},x)}
e^{\ell(y,\hat{Y})}
+
D_{\subtext{KL}}\big(p(\hat{Y}|d_{n},x)\|p(\hat{Y}|d_{n-1},x)\big)
\end{equation}

\textit{Proof}.

\begin{equation}
\begin{split}
D_{\subtext{KL}}\big(p(\hat{Y}|d_{n},x)\|p(\hat{Y}|d_{n-1},x)\big)
&=
\textstyle\sup_{\ell':\mathcal{Y}^{2}\rightarrow\mathbb{R}}
\big\{
\mathbb{E}_{\hat{Y}\sim p(\cdot|d_{n},x)}
\ell'(y,\hat{Y})
-
\log
\mathbb{E}_{\hat{Y}\sim p(\cdot|d_{n-1},x)}
e^{\ell'(y,\hat{Y})}
\big\}
\\
&\geq
\mathbb{E}_{\hat{Y}\sim p(\cdot|d_{n},x)}
\ell(y,\hat{Y})
-
\log
\mathbb{E}_{\hat{Y}\sim p(\cdot|d_{n-1},x)}
e^{\ell(y,\hat{Y})}
\\
\log
\mathbb{E}_{\hat{Y}\sim p(\cdot|d_{n-1},x)}
e^{\ell(y,\hat{Y})}
&=
\textstyle\sup_{p'\in\Delta(\mathcal{Y})}\big\{
\mathbb{E}_{\hat{Y}\sim p'}
\ell(y,\hat{Y})
-
D_{\subtext{KL}}\big(p'\|p(\hat{Y}|d_{n-1},x)\big)
\big\}
\\
&\geq
\mathbb{E}_{\hat{Y}\sim p(\cdot|d_{n},x)}
\ell(y,\hat{Y})
-
D_{\subtext{KL}}\big(p(\hat{Y}|d_{n},x)\|p(\hat{Y}|d_{n-1},x)\big)
\end{split}
\end{equation}

%==============================================================================
\textbf{Lemma}.
%==============================================================================

\begin{equation}
\log
\mathbb{E}_{\hat{Y}\sim p(\cdot|d_{n},x)}
e^{\lambda\ell(y,\hat{Y})}
-
\mathbb{E}_{\hat{Y}\sim p(\cdot|d_{n},x)}
\lambda\ell(y,\hat{Y})
\leq
(e^{(b-a)\lambda}-(b-a)\lambda-1)
\mathbb{E}_{\hat{Y}\sim p(\cdot|d_{n},x)}
\tfrac{\ell(y,\hat{Y})^{2}}{(b-a)^{2}}
\end{equation}

\textit{Proof}.

\begin{equation}
\begin{split}
e^{\lambda\ell(y,\hat{y})}-\lambda\ell(y,\hat{y})-1
&\leq
(e^{(b-a)\lambda}-(b-a)\lambda-1)
\tfrac{\ell(y,\hat{y})^{2}}{(b-a)^{2}}
\\
\mathbb{E}_{\hat{Y}\sim p(\cdot|d_{n},x)}[e^{\lambda\ell(y,\hat{Y})}-\lambda\ell(y,\hat{Y})-1]
&\leq
(e^{(b-a)\lambda}-(b-a)\lambda-1)
\mathbb{E}_{\hat{Y}\sim p(\cdot|d_{n},x)}
\tfrac{\ell(y,\hat{Y})^{2}}{(b-a)^{2}}
\\
\log
\mathbb{E}_{\hat{Y}\sim p(\cdot|d_{n},x)}
e^{\lambda\ell(y,\hat{Y})}
-
\mathbb{E}_{\hat{Y}\sim p(\cdot|d_{n},x)}
\lambda\ell(y,\hat{Y})
&\leq
(e^{(b-a)\lambda}-(b-a)\lambda-1)
\mathbb{E}_{\hat{Y}\sim p(\cdot|d_{n},x)}
\tfrac{\ell(y,\hat{Y})^{2}}{(b-a)^{2}}
\end{split}
\end{equation}

%==============================================================================
\textbf{Proposition}.
%==============================================================================

\begin{equation}
L_{n}
-
L_{n-1}
\leq
f\big(\mathbb{E}_{X\sim p_{*}}D_{\subtext{KL}}\big(p(\hat{Y}|D_{n},X)\|p(\hat{Y}|D_{n-1},X)\big)\big)
\end{equation}

for some monotonically increasing $f$.

\textit{Proof}.

\begin{equation}
\begin{split}
L_{n}
-
L_{n-1}
&=
l(D_{n})
-
l(D_{n-1})
\\
&=
\mathbb{E}_{X,Y\sim p_{*}}
\mathbb{E}_{\hat{Y}\sim p(\cdot|D_{n},X)}
\lambda\ell(Y,\hat{Y})
-
\mathbb{E}_{X,Y\sim p_{*}}
\mathbb{E}_{\hat{Y}\sim p(\cdot|D_{n-1},X)}
\lambda\ell(Y,\hat{Y})
\\
&\leq
\tfrac{1}{\lambda}
\mathbb{E}_{X,Y\sim p_{*}}
\big(
\log
\mathbb{E}_{\hat{Y}\sim p(\cdot|d_{n-1},x)}
e^{\lambda\ell(y,\hat{Y})}
-
\mathbb{E}_{\hat{Y}\sim p(\cdot|D_{n-1},X)}
\lambda\ell(Y,\hat{Y})
\big)
\\
&~~~~+
\tfrac{1}{\lambda}
\mathbb{E}_{X\sim p_{*}}
D_{\subtext{KL}}\big(p(\hat{Y}|D_{n},X)\|p(\hat{Y}|D_{n-1},X)\big)
\\
&\leq
\tfrac{1}{\lambda}
(e^{(b-a)\lambda}-(b-a)\lambda-1)
\mathbb{E}_{X,Y\sim p_{*}}
\mathbb{E}_{\hat{Y}\sim p(\cdot|D_{n-1},X)}
\tfrac{\ell(Y,\hat{Y})^{2}}{(b-a)^{2}}
\\
&~~~~+
\tfrac{1}{\lambda}
\mathbb{E}_{X\sim p_{*}}
D_{\subtext{KL}}\big(p(\hat{Y}|D_{n},X)\|p(\hat{Y}|D_{n-1},X)\big)
\\
&\leq
\tfrac{1}{\lambda}
\tfrac{c^{2}}{(b-a)^{2}}
(e^{(b-a)\lambda}-(b-a)\lambda-1)
+
\tfrac{1}{\lambda}
\mathbb{E}_{X\sim p_{*}}
D_{\subtext{KL}}\big(p(\hat{Y}|D_{n},X)\|p(\hat{Y}|D_{n-1},X)\big)
\end{split}
\end{equation}

where $c$ is such that $\mathbb{E}_{X,Y\sim p_{*}}\mathbb{E}_{\hat{Y}\sim p(\cdot|d,X)}\ell(Y,\hat{Y})^{2}\leq c^{2}$ for any $d$. Minimize RHS w.r.t. $\lambda$:

\begin{equation}
\begin{split}
\tfrac{c^{2}}{(b-a)^{2}}
((b-a)\lambda e^{(b-a)\lambda}
-
e^{(b-a)\lambda}
+1)
&=
\tfrac{(b-a)^{2}}{c^{2}}
\mathbb{E}_{X\sim p_{*}}
D_{\subtext{KL}}\big(p(\hat{Y}|D_{n},X)\|p(\hat{Y}|D_{n-1},X)\big)
-
1
\\
((b-a)\lambda-1)e^{(b-a)\lambda-1}
&=
\tfrac{(b-a)^{2}}{ec^{2}}
\big(\mathbb{E}_{X\sim p_{*}}D_{\subtext{KL}}\big(p(\hat{Y}|D_{n},X)\|p(\hat{Y}|D_{n-1},X)\big)
-
c^{2}\big)
\\
\lambda
=
\tfrac{1}{b-a}\big(
W_{0}\big(
\tfrac{(b-a)^{2}}{ec^{2}}
&
\big(\mathbb{E}_{X\sim p_{*}}D_{\subtext{KL}}\big(p(\hat{Y}|D_{n},X)\|p(\hat{Y}|D_{n-1},X)\big)
-
c^{2}\big)
\big)
+1
\big)
\end{split}
\end{equation}

Substituting back in:

\begin{equation}
\begin{split}
L_{n}
-
L_{n-1}
&\overset{?}{\leq}
(b-a)(e^{W_{0}(\frac{1}{e}(\mathbb{E}_{X\sim p_{*}}D_{\subtext{KL}}(p(\hat{Y}|D_{n},X)\|p(\hat{Y}|D_{n-1},X))-1))+1}-1)
\end{split}
\end{equation}

\newpage
%%%%%%%%%%%%%%%%%%%%%%%%%%%%%%%%%%%%%%%%%%%%%%%%%%%%%%%%%%%%%%%%%%%%%%%%%%%%%%%
\section*{Mutual Information}
%%%%%%%%%%%%%%%%%%%%%%%%%%%%%%%%%%%%%%%%%%%%%%%%%%%%%%%%%%%%%%%%%%%%%%%%%%%%%%%

%==============================================================================
Expected (over $Y|x$) Reduction in Entropy of $\Theta$ (i.e. how much the $Y|x$'s ``inform'' on $\Theta$):
%==============================================================================

\begin{equation}
\begin{split}
\mathbb{I}[\Theta;Y|d,x]
&=
\mathbb{E}_{Y\sim p(\cdot|d,x)}
D_{\subtext{KL}}\big(p(\Theta|d,x,Y)\|p(\Theta|d)\big)
\\
\mathbb{E}_{Y\sim p(\cdot|d,x)}
\mathbb{E}_{\Theta\sim p(\cdot|d,x,Y)}
\log p(\Theta|d,x,Y)
&-
\mathbb{E}_{Y\sim p(\cdot|d,x)}
\mathbb{E}_{\Theta\sim p(\cdot|d,x,Y)}
\log p(\Theta|d)
\\
\mathbb{E}_{Y\sim p(\cdot|d,x)}
\mathbb{E}_{\Theta\sim p(\cdot|d,x,Y)}
\log p(\Theta|d,x,Y)
&-
\mathbb{E}_{\Theta,Y\sim p(\cdot|d,x)}
\log p(\Theta|d)
\\
\mathbb{E}_{Y\sim p(\cdot|d,x)}
\mathbb{E}_{\Theta\sim p(\cdot|d,x,Y)}
\log p(\Theta|d,x,Y)
&-
\mathbb{E}_{\Theta\sim p(\cdot|d)}
\log p(\Theta|d)
\\
\mathbb{H}[\Theta|d]
&-
\mathbb{E}_{Y\sim p(\cdot|d,x)}
\mathbb{H}[\Theta|d,x,Y]
\end{split}
\end{equation}

Remaining expectations can be done by MC sampling (Q: paired vs. not?):

\begin{equation}
\begin{split}
&
\textstyle\sum_{y\in\mathcal{Y}}
\overbrace{
\mathbb{E}_{\Theta\sim p(\cdot|d)}
p(y|x,\Theta)
}^{p(y|d,x)}
\overbracket{
\mathbb{E}_{\Theta'\sim p(\cdot|d,x,y)}
}^{\text{retrain}}
\log p(\Theta'|d,x,y)
-
\mathbb{E}_{\Theta\sim p(\cdot|d)}
\log p(\Theta|d)
\\
&
\textstyle\sum_{y\in\mathcal{Y}}
\underbrace{
\mathbb{E}_{\Theta\sim p(\cdot|d)}
p(y|x,\Theta)
}_{p(y|d,x)}
\underbracket{
\mathbb{E}_{\Theta'\sim p(\cdot|d,x,y)}
}_{\subtext{retrain}}
\big[
\log p(\Theta'|d,x,y)
-
\log p(\Theta'|d)
\big]
\end{split}
\end{equation}

\newpage
%==============================================================================
Expected (over $\Theta$) Reduction in Entropy of $Y|x$ (i.e. how much the $\Theta$'s ``disagree'' on $Y|x$):
%==============================================================================

\begin{equation}
\begin{split}
\mathbb{I}[Y;\Theta|d,x]
&=
\mathbb{E}_{\Theta\sim p(\cdot|d)}
D_{\subtext{KL}}\big(p(Y|x,\Theta)\|p(Y|d,x)\big)
\\
\mathbb{E}_{\Theta\sim p(\cdot|d)}
\mathbb{E}_{Y\sim p(\cdot|x,\Theta)}
\log p(Y|x,\Theta)
&-
\mathbb{E}_{\Theta\sim p(\cdot|d)}
\mathbb{E}_{Y\sim p(\cdot|x,\Theta)}
\log p(Y|d,x)
\\
\mathbb{E}_{\Theta\sim p(\cdot|d)}
\mathbb{E}_{Y\sim p(\cdot|x,\Theta)}
\log p(Y|x,\Theta)
&-
\mathbb{E}_{Y,\Theta\sim p(\cdot|d,x)}
\log p(Y|d,x)
\\
\mathbb{E}_{\Theta\sim p(\cdot|d)}
\mathbb{E}_{Y\sim p(\cdot|x,\Theta)}
\log p(Y|x,\Theta)
&-
\mathbb{E}_{Y\sim p(\cdot|d,x)}
\log p(Y|d,x)
\\
\mathbb{H}[Y|d,x]
&-
\mathbb{E}_{\Theta\sim p(\cdot|d)}
\mathbb{H}[Y|x,\Theta]
\end{split}
\end{equation}

Remaining expectations can be done by MC sampling (Q: paired vs. not?):

\begin{equation}
\begin{split}
&
\mathbb{E}_{\Theta\sim p(\cdot|d)}
\textstyle\sum_{y\in\mathcal{Y}}
p(y|x,\Theta)
\log p(y|x,\Theta)
-
\textstyle\sum_{y\in\mathcal{Y}}
\overbrace{
\mathbb{E}_{\Theta\sim p(\cdot|d)}
p(y|x,\Theta)
}^{p(y|d,x)}
\log
\overbrace{
\mathbb{E}_{\Theta\sim p(\cdot|d)}
p(y|x,\Theta)
}^{p(y|d,x)}
\\
&
\mathbb{E}_{\Theta\sim p(\cdot|d)}
\textstyle\sum_{y\in\mathcal{Y}}
p(y|x,\Theta)
\big[
\log p(y|x,\Theta)
-
\log
\underbrace{
\mathbb{E}_{\Theta\sim p(\cdot|d)}
p(y|x,\Theta)
}_{p(y|d,x)}
\big]
\end{split}
\end{equation}

\newpage
%==============================================================================
Expected (over $Y|x$) Reduction in Entropy of $Y_{*}|X_{*}$ (i.e. how much the $Y|x$'s ``inform'' on $Y_{*}|X_{*}$):
%==============================================================================

\begin{equation}
\begin{split}
\mathbb{I}[Y_{*};Y|d,x,X_{*}]
\mathbb{E}_{X_{*}\sim p_{*}}
&=
\mathbb{E}_{Y\sim p(\cdot|d,x)}
\mathbb{E}_{X_{*}\sim p_{*}}
D_{\subtext{KL}}\big(p(Y_{*}|d,x,Y,X_{*})\|p(Y_{*}|d,X_{*})\big)
\\
\mathbb{E}_{Y\sim p(\cdot|d,x)}
\mathbb{E}_{X_{*}\sim p_{*}}
\mathbb{E}_{Y_{*}\sim p(\cdot|d,x,Y,X_{*})}
\log p(Y_{*}|d,x,Y,X_{*})
&-
\mathbb{E}_{X_{*}\sim p_{*}}
\mathbb{E}_{Y\sim p(\cdot|d,x)}
\mathbb{E}_{Y_{*}\sim p(\cdot|d,x,Y,X_{*})}
\log p(Y_{*}|d,X_{*})
\\
\mathbb{E}_{Y\sim p(\cdot|d,x)}
\mathbb{E}_{X_{*}\sim p_{*}}
\mathbb{E}_{Y_{*}\sim p(\cdot|d,x,Y,X_{*})}
\log p(Y_{*}|d,x,Y,X_{*})
&-
\mathbb{E}_{X_{*}\sim p_{*}}
\mathbb{E}_{Y_{*},Y\sim p(\cdot|d,x,X_{*})}
\log p(Y_{*}|d,X_{*})
\\
\mathbb{E}_{Y\sim p(\cdot|d,x)}
\mathbb{E}_{X_{*}\sim p_{*}}
\mathbb{E}_{Y_{*}\sim p(\cdot|d,x,Y,X_{*})}
\log p(Y_{*}|d,x,Y,X_{*})
&-
\mathbb{E}_{X_{*}\sim p_{*}}
\mathbb{E}_{Y_{*}\sim p(\cdot|d,X_{*})}
\log p(Y_{*}|d,X_{*})
\\
\mathbb{E}_{X_{*}\sim p_{*}}
\mathbb{H}[Y_{*}|d,X_{*}]
&-
\mathbb{E}_{Y\sim p(\cdot|d,x)}
\mathbb{E}_{X_{*}\sim p_{*}}
\mathbb{H}[Y_{*}|d,x,Y,X_{*}]
\end{split}
\end{equation}

Remaining expectations can be done by MC sampling (Q: paired vs. not?):

\begin{equation}
\begin{split}
&
\textstyle\sum_{y\in\mathcal{Y}}
\overbrace{
\mathbb{E}_{\Theta\sim p(\cdot|d)}
p(y|x,\Theta)
}^{p(y|d,x)}
\mathbb{E}_{X_{*}\sim p_{*}}
\textstyle\sum_{y_{*}\in\mathcal{Y}}
\overbrace{
\overbracket{
\mathbb{E}_{\Theta'\sim p(\cdot|d,x,y)}
}^{\text{retrain}}
p(y_{*}|X_{*},\Theta')
}^{p(y_{*}|d,x,y,X_{*})}
\log
\overbrace{
\overbracket{
\mathbb{E}_{\Theta'\sim p(\cdot|d,x,y)}
}^{\text{retrain}}
p(y_{*}|X_{*},\Theta')
}^{p(y_{*}|d,x,y,X_{*})}
\\
&-
\mathbb{E}_{X_{*}\sim p_{*}}
\textstyle\sum_{y_{*}\in\mathcal{Y}}
\underbrace{
\mathbb{E}_{\Theta\sim p(\cdot|d)}
p(y_{*}|X_{*},\Theta)
}_{p(y_{*}|d,X_{*})}
\log
\underbrace{
\mathbb{E}_{\Theta\sim p(\cdot|d)}
p(y_{*}|X_{*},\Theta)
}_{p(y_{*}|d,X_{*})}
\\
&
\textstyle\sum_{y\in\mathcal{Y}}
\overbrace{
\mathbb{E}_{\Theta\sim p(\cdot|d)}
p(y|x,\Theta)
}^{p(y|d,x)}
\mathbb{E}_{X_{*}\sim p_{*}}
\textstyle\sum_{y_{*}\in\mathcal{Y}}
\overbrace{
\overbracket{
\mathbb{E}_{\Theta'\sim p(\cdot|d,x,y)}
}^{\text{retrain}}
p(y_{*}|X_{*},\Theta')
}^{p(y_{*}|d,x,y,X_{*})}
\big[
\log
\overbrace{
\overbracket{
\mathbb{E}_{\Theta'\sim p(\cdot|d,x,y)}
}^{\text{retrain}}
p(y_{*}|X_{*},\Theta')
}^{p(y_{*}|d,x,y,X_{*})}
\\
&-
\log
\underbrace{
\mathbb{E}_{\Theta\sim p(\cdot|d)}
p(y_{*}|X_{*},\Theta)
}_{p(y_{*}|d,X_{*})}
\big]
\end{split}
\end{equation}

\newpage
%==============================================================================
Expected (over $Y_{*}|X_{*}$) Reduction in Entropy of $Y|x$ (i.e. how much the $Y_{*}|X_{*}$'s ``disagree'' on $Y|x$):
%==============================================================================

\begin{equation}
\begin{split}
\mathbb{E}_{X_{*}\sim p_{*}}
\mathbb{I}[Y;Y_{*}|d,x,X_{*}]
&=
\mathbb{E}_{X_{*}\sim p_{*}}
\mathbb{E}_{Y_{*}\sim p(\cdot|d,X_{*})}
D_{\subtext{KL}}\big(p(Y|d,x,X_{*},Y_{*})\|p(Y|d,x)\big)
\\
\mathbb{E}_{X_{*}\sim p_{*}}
\mathbb{E}_{Y_{*}\sim p(\cdot|d,X_{*})}
\mathbb{E}_{Y\sim p(\cdot|d,x,X_{*},Y_{*})}
\log p(Y|d,x,X_{*},Y_{*})
&-
\mathbb{E}_{X_{*}\sim p_{*}}
\mathbb{E}_{Y_{*}\sim p(\cdot|d,X_{*})}
\mathbb{E}_{Y\sim p(\cdot|d,x,X_{*},Y_{*})}
\log p(Y|d,x)
\\
\mathbb{E}_{X_{*}\sim p_{*}}
\mathbb{E}_{Y_{*}\sim p(\cdot|d,X_{*})}
\mathbb{E}_{Y\sim p(\cdot|d,x,X_{*},Y_{*})}
\log p(Y|d,x,X_{*},Y_{*})
&-
\mathbb{E}_{X_{*}\sim p_{*}}
\mathbb{E}_{Y,Y_{*}\sim p(\cdot|d,x,X_{*})}
\log p(Y|d,x)
\\
\mathbb{E}_{X_{*}\sim p_{*}}
\mathbb{E}_{Y_{*}\sim p(\cdot|d,X_{*})}
\mathbb{E}_{Y\sim p(\cdot|d,x,X_{*},Y_{*})}
\log p(Y|d,x,X_{*},Y_{*})
&-
\mathbb{E}_{X_{*}\sim p_{*}}
\mathbb{E}_{Y\sim p(\cdot|d,x)}
\log p(Y|d,x)
\\
\mathbb{H}[Y|d,x]
&-
\mathbb{E}_{X_{*}\sim p_{*}}
\mathbb{E}_{Y_{*}\sim p(\cdot|d,X_{*})}
\mathbb{H}[Y|d,x,X_{*},Y_{*}]
\end{split}
\end{equation}

Remaining expectations can be done by MC sampling (Q: paired vs. not?):

\begin{equation}
\begin{split}
&
\mathbb{E}_{X_{*}\sim p_{*}}
\textstyle\sum_{y_{*}\in\mathcal{Y}}
\overbrace{
\mathbb{E}_{\Theta\sim p(\cdot|d)}
p(y_{*}|X_{*},\Theta)
}^{p(y_{*}|d,X_{*})}
\textstyle\sum_{y\in\mathcal{Y}}
\overbrace{
\overbracket{
\mathbb{E}_{\Theta'\sim p(\cdot|d,X_{*},y_{*})}
}^{\text{retrain}}
p(y|x,\Theta')
}^{p(y|d,x,X_{*},y_{*})}
\log
\overbrace{
\overbracket{
\mathbb{E}_{\Theta'\sim p(\cdot|d,X_{*},y_{*})}
}^{\text{retrain}}
p(y|x,\Theta')
}^{p(y|d,x,X_{*},y_{*})}
\\
&-
\textstyle\sum_{y\in\mathcal{Y}}
\underbrace{
\mathbb{E}_{\Theta\sim p(\cdot|d)}
p(y|x,\Theta)
}_{p(y|d,x)}
\log
\underbrace{
\mathbb{E}_{\Theta\sim p(\cdot|d)}
p(y|x,\Theta)
}_{p(y|d,x)}
\\
&\mathbb{E}_{X_{*}\sim p_{*}}
\textstyle\sum_{y_{*}\in\mathcal{Y}}
\overbrace{
\mathbb{E}_{\Theta\sim p(\cdot|d)}
p(y_{*}|X_{*},\Theta)
}^{p(y_{*}|d,X_{*})}
\textstyle\sum_{y\in\mathcal{Y}}
\overbrace{
\overbracket{
\mathbb{E}_{\Theta'\sim p(\cdot|d,X_{*},y_{*})}
}^{\text{retrain}}
p(y|x,\Theta')
}^{p(y|d,x,X_{*},y_{*})}
\big[
\log
\overbrace{
\overbracket{
\mathbb{E}_{\Theta'\sim p(\cdot|d,X_{*},y_{*})}
}^{\text{retrain}}
p(y|x,\Theta')
}^{p(y|d,x,X_{*},y_{*})}
\\
&-
\log
\underbrace{
\mathbb{E}_{\Theta\sim p(\cdot|d)}
p(y|x,\Theta)
}_{p(y|d,x)}
\big]
\end{split}
\end{equation}
