# Supplementary material for: Online Decision Mediation
Source: arXiv:2310.18601 source file (2023-10-28)
Supplement: Supplementary file 3 [file AlzheimersDataset_OnlineDirichletModel_NoisyAgent_BaseExpert.tex]

448\pix$\pm$\pix22&615\pix$\pm$\pix30&326\pix$\pm$\pix22\\201\pix$\pm$\pix29&466\pix$\pm$\pix22&330\pix$\pm$\pix14\\305\pix$\pm$\pix29&333\pix$\pm$\pix21&333\pix$\pm$\pix21\\275\pix$\pm$\pix20&603\pix$\pm$\pix19&379\pix$\pm$\pix24\\277\pix$\pm$\pix24&665\pix$\pm$\pix35&430\pix$\pm$\pix17\\260\pix$\pm$\pix31&337\pix$\pm$\pix21&290\pix$\pm$\pix20\\220\pix$\pm$\pix21&284\pix$\pm$\pix13&265\pix$\pm$\pix15\\177\pix$\pm$\pix22&449\pix$\pm$\pix25&275\pix$\pm$\pix17\\143\pix$\pm$\pix16&351\pix$\pm$\pix18&238\pix$\pm$\pix16\\128\pix$\pm$\pix12&211\pix$\pm$\pix17&175\pix$\pm$\pix14\\\midrule90\pix$\pm$\pix12&130\pix$\pm$\pix18&125\pix$\pm$\pix11\\
