# Supplementary material for: Online Decision Mediation
Source: arXiv:2310.18601 source file (2023-10-28)
Supplement: Supplementary file 4 [file CysticFibrosisDataset_OnlineDirichletModel_NoisyAgent_BaseExpert.tex]

448\pix$\pm$\pix22&616\pix$\pm$\pix23&325\pix$\pm$\pix20\\155\pix$\pm$\pix23&536\pix$\pm$\pix46&344\pix$\pm$\pix22\\265\pix$\pm$\pix16&299\pix$\pm$\pix19&296\pix$\pm$\pix11\\284\pix$\pm$\pix13&628\pix$\pm$\pix32&374\pix$\pm$\pix21\\273\pix$\pm$\pix24&714\pix$\pm$\pix33&450\pix$\pm$\pix13\\226\pix$\pm$\pix24&315\pix$\pm$\pix23&267\pix$\pm$\pix19\\167\pix$\pm$\pix22&275\pix$\pm$\pix27&234\pix$\pm$\pix12\\136\pix$\pm$\pix19&429\pix$\pm$\pix22&248\pix$\pm$\pix21\\114\pix$\pm$\pix26&371\pix$\pm$\pix24&232\pix$\pm$\pix20\\93\pix$\pm$\pix11&198\pix$\pm$\pix21&155\pix$\pm$\pix12\\\midrule80\pix$\pm$\pix13&132\pix$\pm$\pix12&119\pix$\pm$\pix15\\
