# Supplementary material for: Online Decision Mediation
Source: arXiv:2310.18601 source file (2023-10-28)
Supplement: Supplementary file 5 [file GaussSineDataset_OnlineDirichletModel_NoisyAgent_BaseExpert.tex]

116\pix$\pm$\pix8&131\pix$\pm$\pix7&37\pix$\pm$\pix8\\19\pix$\pm$\pix8&47\pix$\pm$\pix7&34\pix$\pm$\pix7\\33\pix$\pm$\pix14&36\pix$\pm$\pix11&37\pix$\pm$\pix11\\44\pix$\pm$\pix10&90\pix$\pm$\pix18&50\pix$\pm$\pix10\\41\pix$\pm$\pix7&105\pix$\pm$\pix14&64\pix$\pm$\pix7\\29\pix$\pm$\pix9&42\pix$\pm$\pix11&28\pix$\pm$\pix11\\16\pix$\pm$\pix7&25\pix$\pm$\pix7&22\pix$\pm$\pix4\\16\pix$\pm$\pix7&45\pix$\pm$\pix9&26\pix$\pm$\pix7\\12\pix$\pm$\pix6&25\pix$\pm$\pix7&19\pix$\pm$\pix4\\15\pix$\pm$\pix6&23\pix$\pm$\pix8&20\pix$\pm$\pix4\\\midrule4\pix$\pm$\pix3&6\pix$\pm$\pix3&6\pix$\pm$\pix4\\
