# Supplementary material for: Online Decision Mediation
Source: arXiv:2310.18601 source file (2023-10-28)
Supplement: Supplementary file 6 [file HandGesturesDataset_OnlineDirichletModel_NoisyAgent_BaseExpert.tex]

454\pix$\pm$\pix18&572\pix$\pm$\pix24&260\pix$\pm$\pix21\\39\pix$\pm$\pix8&485\pix$\pm$\pix34&256\pix$\pm$\pix14\\101\pix$\pm$\pix36&352\pix$\pm$\pix48&232\pix$\pm$\pix41\\118\pix$\pm$\pix14&622\pix$\pm$\pix18&303\pix$\pm$\pix10\\119\pix$\pm$\pix18&728\pix$\pm$\pix32&415\pix$\pm$\pix28\\95\pix$\pm$\pix28&319\pix$\pm$\pix66&194\pix$\pm$\pix47\\32\pix$\pm$\pix6&220\pix$\pm$\pix31&132\pix$\pm$\pix15\\41\pix$\pm$\pix19&441\pix$\pm$\pix39&194\pix$\pm$\pix31\\19\pix$\pm$\pix6&232\pix$\pm$\pix26&125\pix$\pm$\pix14\\21\pix$\pm$\pix4&158\pix$\pm$\pix23&93\pix$\pm$\pix13\\\midrule13\pix$\pm$\pix5&67\pix$\pm$\pix28&42\pix$\pm$\pix17\\
