# Supplementary material for: Online Decision Mediation
Source: arXiv:2310.18601 source file (2023-10-28)
Supplement: Supplementary file 7 [file LunarLanderDataset_OnlineDirichletModel_NoisyAgent_BaseExpert.tex]

449\pix$\pm$\pix18&634\pix$\pm$\pix21&386\pix$\pm$\pix26\\114\pix$\pm$\pix18&661\pix$\pm$\pix39&388\pix$\pm$\pix27\\166\pix$\pm$\pix20&607\pix$\pm$\pix36&403\pix$\pm$\pix18\\202\pix$\pm$\pix39&882\pix$\pm$\pix79&502\pix$\pm$\pix63\\205\pix$\pm$\pix28&907\pix$\pm$\pix43&552\pix$\pm$\pix31\\172\pix$\pm$\pix19&587\pix$\pm$\pix24&385\pix$\pm$\pix21\\129\pix$\pm$\pix19&523\pix$\pm$\pix42&342\pix$\pm$\pix26\\111\pix$\pm$\pix18&704\pix$\pm$\pix47&364\pix$\pm$\pix30\\87\pix$\pm$\pix11&532\pix$\pm$\pix26&304\pix$\pm$\pix19\\102\pix$\pm$\pix12&449\pix$\pm$\pix23&291\pix$\pm$\pix16\\\midrule64\pix$\pm$\pix12&343\pix$\pm$\pix16&212\pix$\pm$\pix15\\
