# Supplementary material for: Online Decision Mediation
Source: arXiv:2310.18601 source file (2023-10-28)
Supplement: Supplementary file 8 [file MagicGammaDataset_OnlineDirichletModel_NoisyAgent_BaseExpert.tex]

452\pix$\pm$\pix17&545\pix$\pm$\pix19&199\pix$\pm$\pix11\\204\pix$\pm$\pix17&201\pix$\pm$\pix20&203\pix$\pm$\pix18\\176\pix$\pm$\pix15&139\pix$\pm$\pix16&176\pix$\pm$\pix15\\229\pix$\pm$\pix24&226\pix$\pm$\pix17&194\pix$\pm$\pix20\\231\pix$\pm$\pix10&252\pix$\pm$\pix14&219\pix$\pm$\pix9\\196\pix$\pm$\pix20&177\pix$\pm$\pix28&174\pix$\pm$\pix20\\162\pix$\pm$\pix13&124\pix$\pm$\pix14&162\pix$\pm$\pix13\\139\pix$\pm$\pix14&147\pix$\pm$\pix10&143\pix$\pm$\pix14\\191\pix$\pm$\pix14&192\pix$\pm$\pix18&192\pix$\pm$\pix13\\154\pix$\pm$\pix11&122\pix$\pm$\pix12&154\pix$\pm$\pix11\\\midrule112\pix$\pm$\pix15&86\pix$\pm$\pix9&112\pix$\pm$\pix15\\
