# Supplementary material for: Online Decision Mediation
Source: arXiv:2310.18601 source file (2023-10-28)
Supplement: Supplementary file 9 [file AlzheimersDataset_OnlineDirichletModel_NoisyAgent_BaseExpert.tex]

706\pix$\pm$\pix83&250\pix$\pm$\pix114&541\pix$\pm$\pix96\\305\pix$\pm$\pix29&333\pix$\pm$\pix21&333\pix$\pm$\pix21\\258\pix$\pm$\pix33&375\pix$\pm$\pix27&330\pix$\pm$\pix14\\220\pix$\pm$\pix21&284\pix$\pm$\pix13&265\pix$\pm$\pix15\\198\pix$\pm$\pix14&333\pix$\pm$\pix23&265\pix$\pm$\pix15\\128\pix$\pm$\pix12&211\pix$\pm$\pix17&175\pix$\pm$\pix14\\\midrule90\pix$\pm$\pix12&130\pix$\pm$\pix18&125\pix$\pm$\pix11\\
