# Supplementary material for: Online Decision Mediation
Source: arXiv:2310.18601 source file (2023-10-28)
Supplement: Supplementary file 10 [file CysticFibrosisDataset_OnlineDirichletModel_NoisyAgent_BaseExpert.tex]

714\pix$\pm$\pix53&285\pix$\pm$\pix78&580\pix$\pm$\pix48\\265\pix$\pm$\pix16&299\pix$\pm$\pix19&296\pix$\pm$\pix11\\264\pix$\pm$\pix27&374\pix$\pm$\pix52&344\pix$\pm$\pix22\\167\pix$\pm$\pix22&275\pix$\pm$\pix27&234\pix$\pm$\pix12\\180\pix$\pm$\pix28&313\pix$\pm$\pix26&256\pix$\pm$\pix19\\93\pix$\pm$\pix11&198\pix$\pm$\pix21&155\pix$\pm$\pix12\\\midrule70\pix$\pm$\pix11&120\pix$\pm$\pix11&106\pix$\pm$\pix12\\
