# Supplementary material for: Online Decision Mediation
Source: arXiv:2310.18601 source file (2023-10-28)
Supplement: Supplementary file 11 [file GaussSineDataset_OnlineDirichletModel_NoisyAgent_BaseExpert.tex]

124\pix$\pm$\pix33&84\pix$\pm$\pix40&120\pix$\pm$\pix34\\33\pix$\pm$\pix14&36\pix$\pm$\pix11&37\pix$\pm$\pix11\\29\pix$\pm$\pix10&32\pix$\pm$\pix7&34\pix$\pm$\pix7\\16\pix$\pm$\pix7&25\pix$\pm$\pix7&22\pix$\pm$\pix4\\19\pix$\pm$\pix5&21\pix$\pm$\pix6&23\pix$\pm$\pix5\\15\pix$\pm$\pix6&23\pix$\pm$\pix8&20\pix$\pm$\pix4\\\midrule4\pix$\pm$\pix3&6\pix$\pm$\pix3&6\pix$\pm$\pix4\\
