# Supplementary material for: Online Decision Mediation
Source: arXiv:2310.18601 source file (2023-10-28)
Supplement: Supplementary file 12 [file HandGesturesDataset_OnlineDirichletModel_NoisyAgent_BaseExpert.tex]

530\pix$\pm$\pix60&397\pix$\pm$\pix71&589\pix$\pm$\pix40\\101\pix$\pm$\pix36&352\pix$\pm$\pix48&232\pix$\pm$\pix41\\81\pix$\pm$\pix12&386\pix$\pm$\pix32&256\pix$\pm$\pix14\\32\pix$\pm$\pix6&220\pix$\pm$\pix31&132\pix$\pm$\pix15\\48\pix$\pm$\pix11&290\pix$\pm$\pix31&187\pix$\pm$\pix18\\21\pix$\pm$\pix4&158\pix$\pm$\pix23&93\pix$\pm$\pix13\\\midrule13\pix$\pm$\pix5&67\pix$\pm$\pix28&42\pix$\pm$\pix17\\
