# Supplementary material for: Online Decision Mediation
Source: arXiv:2310.18601 source file (2023-10-28)
Supplement: Supplementary file 13 [file LunarLanderDataset_OnlineDirichletModel_NoisyAgent_BaseExpert.tex]

596\pix$\pm$\pix171&538\pix$\pm$\pix165&681\pix$\pm$\pix79\\166\pix$\pm$\pix20&607\pix$\pm$\pix36&403\pix$\pm$\pix18\\161\pix$\pm$\pix21&568\pix$\pm$\pix37&388\pix$\pm$\pix27\\129\pix$\pm$\pix19&523\pix$\pm$\pix42&342\pix$\pm$\pix26\\130\pix$\pm$\pix19&540\pix$\pm$\pix26&345\pix$\pm$\pix27\\102\pix$\pm$\pix12&449\pix$\pm$\pix23&291\pix$\pm$\pix16\\\midrule64\pix$\pm$\pix12&343\pix$\pm$\pix16&212\pix$\pm$\pix15\\
