# Supplementary material for: Online Decision Mediation
Source: arXiv:2310.18601 source file (2023-10-28)
Supplement: Supplementary file 14 [file MagicGammaDataset_OnlineDirichletModel_NoisyAgent_BaseExpert.tex]

581\pix$\pm$\pix65&400\pix$\pm$\pix140&493\pix$\pm$\pix106\\176\pix$\pm$\pix15&139\pix$\pm$\pix16&176\pix$\pm$\pix15\\227\pix$\pm$\pix16&176\pix$\pm$\pix17&203\pix$\pm$\pix18\\162\pix$\pm$\pix13&124\pix$\pm$\pix14&162\pix$\pm$\pix13\\212\pix$\pm$\pix13&174\pix$\pm$\pix14&194\pix$\pm$\pix12\\154\pix$\pm$\pix11&122\pix$\pm$\pix12&154\pix$\pm$\pix11\\\midrule112\pix$\pm$\pix15&86\pix$\pm$\pix9&112\pix$\pm$\pix15\\
