# Supplementary material for: Online Decision Mediation
Source: arXiv:2310.18601 source file (2023-10-28)
Supplement: Supplementary file 15 [file referees.tex]

\tttext{No Requuest}\\\tttext{Passive Request}\\\tttext{Epsilon-Request w/o CS}\\\tttext{Epsilon-Request with CS}\\\tttext{Dynamic-Request w.p.~KG}\\\tttext{Dynamic-Request with ME}\\\midrule\textbf{UMPIRE}\\
